# Supplementary material for: Interaction of ultraintense radially-polarized laser pulses with plasma mirrors
Source: arXiv:2004.03645 source file (2020-04-07)
Supplement: Supplementary file 1 [file SupplementalMaterial.pdf]

# Supplemental material for: Interaction of ultraintense radially-polarized laser pulses with plasma mirrors

N. Zaïm[1], D. Guénot[1,2], L. Chopineau[3], A. Denoeud[3],
O. Lundh[2], H. Vincenti[3], F. Quéré[3] and J. Faure[1]

[1] *LOA, CNRS, École Polytechnique, ENSTA Paris, Institut Polytechnique de Paris, 181 Chemin de la Hunière et des Joncherettes, 91120 Palaiseau, France*

[2] *Department of physics, Lund University, SE-22100 Lund, Sweden*

[3] *Lasers, Interactions and Dynamics Laboratory (LIDyL), Commissariat à l'Énergie Atomique, Université Paris-Saclay, DSM/IRAMIS, CEN Saclay, 91191 Gif sur Yvette, France*

## I. PARAMETERS FOR THE 3D PIC SIMULATIONS

We use a spatial resolution of $\Delta x = \Delta y = \Delta z = \lambda_0/57$, a temporal resolution of $\Delta t = T_0/57$ and 6 particles per cell per specie. The PSATD Maxwell solver is used with a stencil spatial order of 100 and 8 guard cells. The laser impinges the plasma with a 60° incidence angle, a central wavelength of $\lambda_0 = 800$ nm, a beam waist of $w_0 = 3.1\,\mu$m and a pulse duration of 24 fs in FWHM of intensity. The peak normalized amplitude of the transverse field is $a_0 = 5.4$ for linear polarization and $a_{0,r} = 4.9$ for radial and azimuthal polarization. The intensity was reduced to obtain the accelerated electron distributions, as indicated in the main text. A cosine temporal envelope is used. The plasma density profile is exponential with a minimum density of $n_c/20$ and a maximum density of 100 $n_c$. The gradient scale length is $L = \lambda_0/10$, except in the simulations at reduced intensity in radial and azimuthal polarization, where it is $L = \lambda_0/7$.

## II. PARAMETERS FOR THE TEST PARTICLE SIMULATION

We use in the test particle simulation a laser pulse with the same spatio-temporal profile as in Ref. [1]. We use a central wavelength of $\lambda_0 = 800$ nm, a beam waist of $w_0 = 3.1\,\mu$m, a pulse duration of 24 fs in FWHM of intensity and a peak normalized amplitude of the radial electric field of $a_{0,r} = 2.6$ or $a_{0,r} = 1.3$. These values are slightly lower than in the PIC simulations to take into account the fact that the reflectivity of the plasma mirror is smaller than unity.

The initial electron distributions are as indicated in the main text.

## III. PARAMETERS FOR THE PIC SIMULATION IN CYLINDRICAL COORDINATES

We use a spatial resolution of $\Delta x = \lambda_0/279$ and $\Delta r = \lambda_0/65$, a temporal resolution of $\Delta t = T_0/331$, 250 particles per cell per specie and 2 orders for the Fourier expansion along the azimuthal direction. The plasma density profile is exponential with a gradient scale length of $L = \lambda_0/7$, a minimum density of $n_c/10$ and a maximum density of 200 $n_c$. The laser has a central wavelength of $\lambda_0 = 800$ nm, a beam waist of $w_0 = 1.5\,\mu$m and a pulse duration of 5 fs in FWHM of intensity. The peak normalized amplitude of the longitudinal field is $a_{0,z} = 3.78$ and the peak amplitude of the radial field is $a_{0,r} = 9.55$

for radial and azimuthal polarization. We use the same laser spatio-temporal profile as in Ref. [1].


[1] V. Marceau, C. Varin, T. Brabec, and M. Piché. Femtosecond 240-keV electron pulses from direct laser acceleration in a low-density gas. *Phys. Rev. Lett.*, 111(22):224801, 2013.
